# Supplementary material for: Electrically Controlled Spin Injection from Giant Rashba Spin-Orbit Conductor BiTeBr
Source: arXiv:2008.13764 ancillary file (2020-08-31)
Supplement: Supplementary file 1 [file Supporting_Information.pdf]

# Supporting Information:
## Electrically Controlled Spin Injection from Giant Rashba Spin-Orbit Conductor BiTeBr

Zoltán Kovács-Krausz,[1] Anamul Md Hoque,[2] Péter Makk,[1,*] Bálint Szentpéteri,[1] Mátyás Kocsis,[1] Bálint Fülöp,[1] Michael Vasilievich Yakushev,[3,4,5] Tatyana Vladimirovna Kuznetsova,[3,4] Oleg Evgenevich Tereshchenko,[6,7,8] Konstantin Aleksandrovich Kokh,[6,8,9] István Endre Lukács,[10] Takashi Taniguchi,[11] Kenji Watanabe,[11] Saroj Prasad Dash,[2,†] and Szabolcs Csonka[1]

[1]*Department of Physics, Budapest University of Technology and Economics and Nanoelectronics 'Momentum' Research Group of the Hungarian Academy of Sciences, Budafoki ut 8, 1111 Budapest, Hungary*
[2]*Department of Microtechnology and Nanoscience, Chalmers University of Technology, SE-41296, Göteborg, Sweden*
[3]*M.N. Miheev Institute of Metal Physics of UB RAS, 620108, Ekaterinburg, Russia.*
[4]*Ural Federal University, Ekaterinburg, 620002, Russia.*
[5]*Institute of Solid State Chemistry of UB RAS, Ekaterinburg, 620990, Russia.*
[6]*St. Petersburg State University, 198504, St. Petersburg, Russia.*
[7]*A.V. Rzhanov Institute of Semiconductor Physics, 630090, Novosibirsk, Russia.*
[8]*Novosibirsk State University, 630090, Novosibirsk, Russia.*
[9]*V.S. Sobolev Institute of Geology and Mineralogy, 630090, Novosibirsk, Russia.*
[10]*Center for Energy Research, Institute of Technical Physics and Material Science, H-1121 Budapest, Hungary*
[11]*National Institute for Material Science, 1-1 Namiki, Tsukuba, 305-0044, Japan*

## S I. DEVICE FABRICATION AND EXPERIMENTAL METHODS

Single crystals of BiTeBr were grown by a modified Bridgman method with rotating heat field [1]. Mixtures of binary compounds $Bi_2Te_3$ and $BiBr_3$ were used as charges to grow BiTeBr. According to Ref. [2] BiTeBr has a congruent melting point at 526° C. Therefore a stoichiometric charge of the binary compounds was used to grow BiTeBr. Charges, sealed under vacuum in quartz ampoules, were at first prereacted at temperatures exceeding the melting points by 20° C and then pulled through vertical gradient of 15° C/cm at a rate of 10 mm/day. More technical details can be found in Refs [1, 3].

Graphene was exfoliated to a Si/$SiO_2$ chip with approximately 290 nm oxide thickness, that had been treated with 10 min UVO exposure immediately before exfoliation. For some devices (e.g. Device 2), graphene was instead dry-transferred onto a hexagonal boron-nitride (hBN) substrate on a similar Si/$SiO_2$ chip. BiTeBr was exfoliated directly to a clean polydimethylsiloxane (PDMS) layer. The exfoliation to PDMS was performed at a reduced ambient temperature of 5 °C, as AFM imaging confirmed a significant reduction of glue residue on the BiTeBr compared to room temperature exfoliation. 40-100 nm thick crystals few-μm in lateral dimensions were selected. The presence of atomically flat steps on these crystals was observed by AFM. To create the BiTeBr-graphene device, the crystals were dry-transferred, with the help of the PDMS substrate, onto the previously exfoliated graphene flakes.

FM contacts were created via electron beam lithography and electron beam vapor deposition of metallic Co (80 nm). Varying contact widths between 200-300 nm were used to create different coercive fields for the FM switching. For easy readout of non-local spin signals, graphene channel lengths of 2-6 μm were left between contacts. Tunnel barriers were first deposited to enhance the otherwise low efficiency of spin injection caused by a conductivity mismatch between Co and graphene. The $TiO_2$ tunnel barriers were grown using two repeated steps of 0.5 nm Ti deposition and low pressure oxidation. Conventional metallic contacts on top of BiTeBr were also fabricated similarly, using a 10 nm Cr adhesion layer followed by 80 nm Au. The BiTeBr surface was cleaned using low power Ar plasma milling right before deposition.

Charge and spin transport measurements on the samples were performed at room temperature using a Helmholtz coil to apply magnetic fields up to 0.8 T. The sample environment was held under vacuum to prevent oxidation of the FM contacts. The electrical measurements were performed using DC current bias. The Si substrate under the 290 nm $SiO_2$ layer was used as a global backgate electrode.

* E-mail: peter.makk@mail.bme.hu
† E-mail: saroj.dash@chalmers.se

## S II. DEVICE 1 CHARACTERIZATION

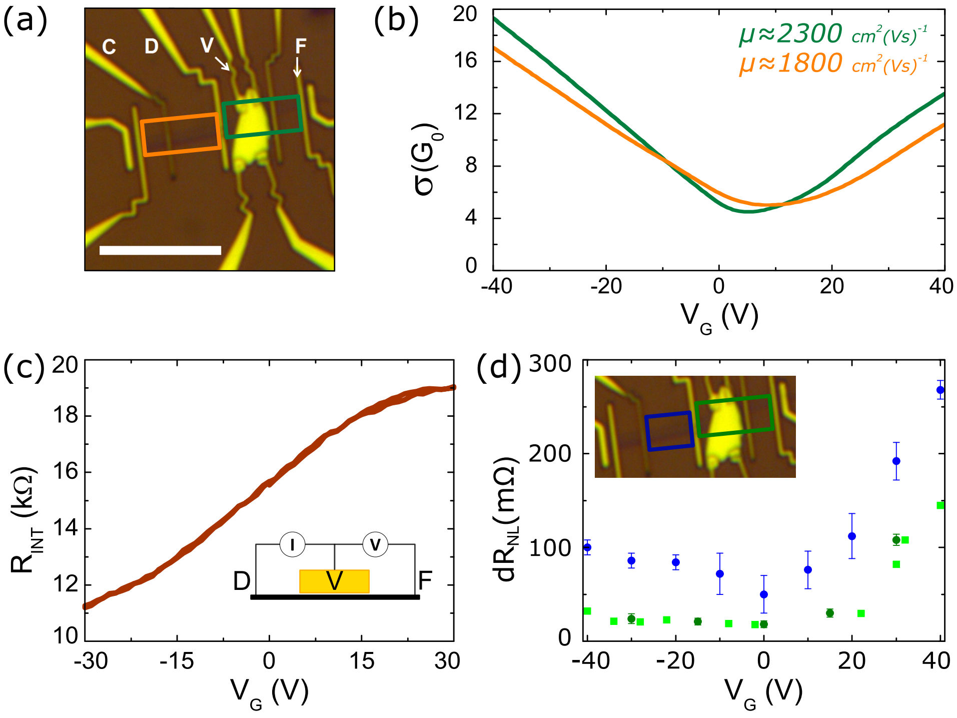


Figure S1. (a) An optical image of Device 1, with colors indicating sections investigated for charge transport. Scale bar is 10 µm. (b) Conductivity of the same sections and extracted mobility. (c) Gate dependence of interface resistance between BiTeBr and graphene under vertical current bias. (d) Spin transport. The magnitude of the switching $dR_{\mathrm{NL}}$ as a function of gate voltage, for the bare graphene section (blue) and section containing BiTeBr (green). For the latter, circles represent data from non-local spin valve measurements, while squares are the same information extracted from Hanle spin precession measurements. The spin relaxation dynamics are similar for the sections. There is an electron-hole asymmetry in the signal, caused by pinholes in the FM tunnel barriers.

Charge and spin transport measurements for the first device are presented in addition to those found in Fig. 2 of the main text. For evaluation of charge transport in the graphene detector circuit and the effect of the BiTeBr, similarly sized graphene sections of the device were chosen as depicted by the green and orange sections in Fig. S1 (a). The four-terminal resistances as function of gate voltage are shown in Fig. 2 (b) of the main text, for the corresponding sections in the same colors. The charge neutrality points $V_{\mathrm{CNP}}$ are similar, being 12 V for the reference graphene section and 6 V for the section partially covered by BiTeBr. On Fig. S1 (b) the conductivity of the same section is shown, with extracted mobilities $\mu$ of $1800\,\mathrm{cm^2(Vs)^{-1}}$ and $2300\,\mathrm{cm^2(Vs)^{-1}}$ respectively.

By modeling the graphene, $SiO_2$ dielectric (approximately 290 nm) and Si backgate as a capacitor, graphene charge carrier density can be obtained, and by plotting the conductivity data on a log-log scale, a residual doping $n_{\mathrm{RES}}$ of $7.0\times10^{15}\,\mathrm{m^{-2}}$ and $5.5\times10^{15}\,\mathrm{m^{-2}}$ is obtained for the reference and BiTeBr covered sections, respectively. A diffusion coefficient at $V_{\mathrm{CNP}}$ of $101\,\mathrm{cm^2s^{-1}}$ and $93\,\mathrm{cm^2s^{-1}}$, respectively, is calculated by the formula

$$D(V_{\mathrm{G}}) = \frac{\hbar v_{\mathrm{F}}\mu}{2e}\sqrt{\pi\sqrt{n^2\left(V_{\mathrm{G}}\right)+n_{\mathrm{RES}}^2}}, \tag{S1}$$

which takes into account residual doping [4], since $n\left(V_{\mathrm{CNP}}\right)=0$ for ideal graphene.

On Fig. S1 (c) the gate dependence of the BiTeBr-graphene interface is shown, measured in a three-terminal setup (contacts D-V for current bias and V-F for voltage sensing), while the resistances of the BiTeBr crystal and the metallic top contact have negligible contributions on the order of 100Ω. The interface resistance is modestly tunable, but at all gate voltages it is significantly larger than the graphene $R_{\mathrm{sq}}\approx 2.2\ \mathrm{k\Omega}$, which is consistent with the BiTeBr crystal not having significant proximity-induced influence on graphene spin transport. Charge transport is also unaffected, as evidenced by the similar $V_{\mathrm{CNP}}$, mobility, residual doping, and diffusion coefficient of the sections. For comparison,

in studies where proximity-based spin transport is found to be affected, typically in TMDC/graphene structures, interfaces are found to be of similar or lower resistance than graphene $R_{sq}$ [5–8].

The methodology for extracting spin transport characteristics is detailed further below, and the values are summarized in Table II. We may note that the obtained spin diffusion coefficient $D_S$ is comparable to the charge diffusion coefficient $D$ obtained here.

Finally, Fig. S1 (d) shows the non-local (NL) resistance $dR_{NL}$, obtained from NL spin valve and Hanle spin precession measurements, plotted as a function of gate voltage, for the sections indicated by the inset. Once again, similar behavior is observed for the BiTeBr-containing and reference graphene channels. There is an electron-hole asymmetry in the signal amplitude, potentially caused by the presence of pinholes in the oxide barriers of FM contacts [9–11]. The resistances at the FM/$TiO_2$/graphene interface are in the same order of magnitude as the graphene $R_{sq}$, with contact resistances $R_C = 2.3\,k\Omega$, $R_D = 3.9\,k\Omega$ and $R_F = 0.6\,k\Omega$ of contacts C,D and F respectively. Slight decreases in these values were observed after passing current through these contacts, further indicating pinhole-type defects in the barriers.

## S III. DEVICE 2 CHARACTERIZATION

The second device, which is mentioned in Fig. 4 of the main text, is detailed here. This device was fabricated similarly to Device 1, as detailed in the Methods section, except this device was placed on a hexagonal boron nitride (hBN) substrate previously exfoliated to the $SiO_2$, similarly to Ref. [12]. The presence of the hBN (visible in the background in Fig. S2 (a)) did not have any notable impact on device behavior other than a modest increase in spin relaxation time as mentioned below.

Fig. S2 (b) shows the NL spin valve measurement between contacts E-F on the device, with E serving as current injector towards a more distant graphene contact, A. The FM contact magnetization switching leads to the observed single jumps in the signal while sweeping the magnetic field $B_Y$ up and down, as described in the main text in Fig. 3.

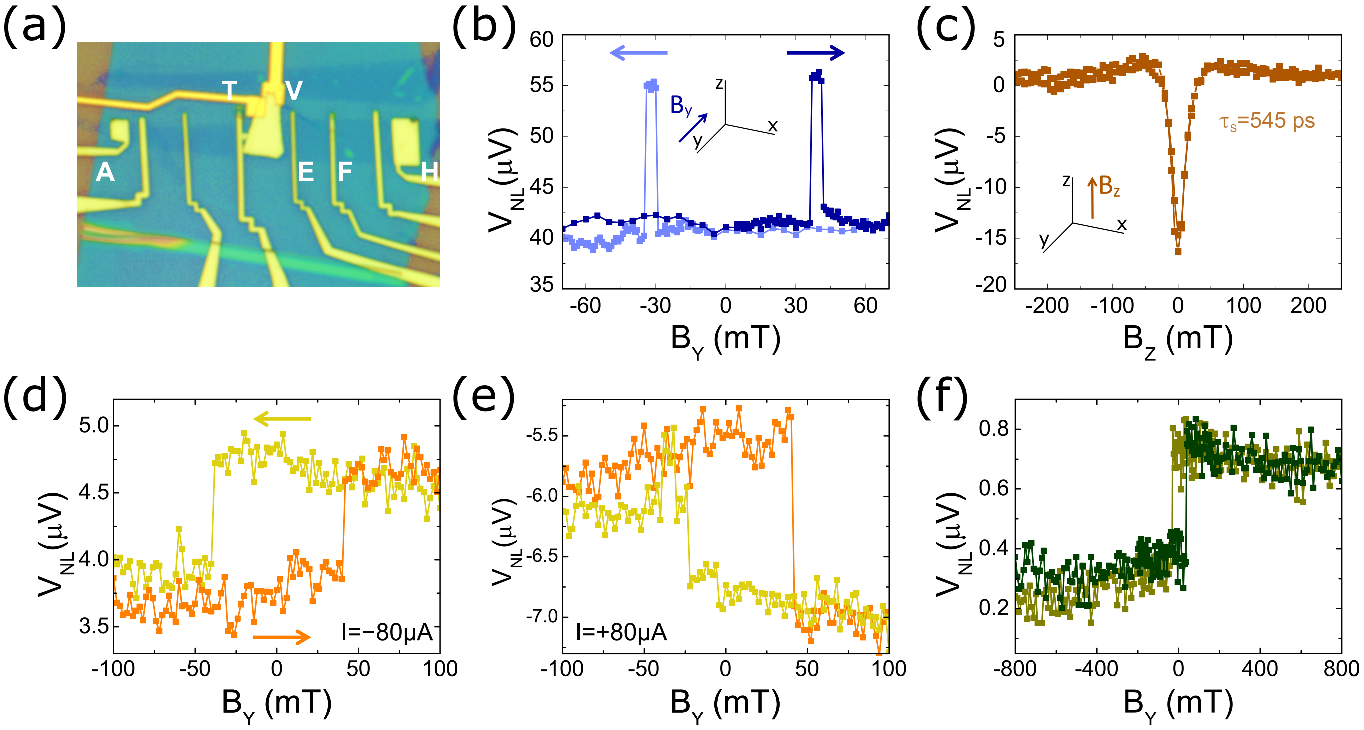


Figure S2. (a) Optical image of Device 2, where the section between contacts E-F was used as a reference graphene channel. (b) Non-local spin valve measurement on the reference graphene channel, showing the switching in non-local voltage while sweeping the field $B_Y$. (c) Curve obtained from Hanle spin precession in the reference graphene channel while sweeping the out-of-plane field $B_Z$, with extracted spin relaxation time. (d) & (e) Signal originating in bulk BiTeBr by using contact V as injector and F as detector. The direction of sweeping magnetic field is shown by horizontal arrows. There is only one transition observed in each direction, that of the FM detector's magnetization. The same measurements shown for $\pm 80$ μA bias current. (f) Similar signal demonstrating the absence of any second switch up to 800 mT.

Subpanel (c), shows Hanle spin precession using the same contacts, and an out-of-plane field, $B_Z$. Fitting of the Hanle curve using Eq. S3 results in $\tau_S = 545\,\mathrm{ps}$ and $D_S = 110\,\mathrm{cm^2 s^{-1}}$, resulting in $\lambda_S = 2.5\,\mathrm{\mu m}$. Other than the modestly higher $\tau_S$, these values are comparable to those in Device 1.

Measured between contacts E-F also, the graphene channel in Device 2 has $R_{sq} = 1.2\,\mathrm{k\Omega}$, while three-terminal measurements of the BiTeBr-graphene interface result in $R_{INT} = 8.3\,\mathrm{k\Omega}$. Measuring resistance of the BiTeBr crystal between contacts T-V, we obtain $109\,\Omega$. FM tunnel barrier contact resistances $R_E$ and $R_F$ are approximately $14\,\mathrm{k\Omega}$. This is greater than $R_{sq}$, which might explain the higher $\tau_S$ value compared to Device 1 [9].

Fig. S2 (d) & (e) show the NL spin signal while using BiTeBr as an injector, using contact V, and distant reference contact A on the graphene. Detection takes place on FM contact F. The resulting switching behavior with magnetic field, like in Fig. 3 of the main text, is consistent with REE in bulk BiTeBr, with polarization injected into graphene and diffusing toward the FM detector. The orientation of the injected spins depends on the in-plane electric field $E_{IP}$ inside BiTeBr, and doesn't change with sweeping $B_Y$, therefore only a single switch attributable to contact F is seen, at the same coercive field as in the measurement in subpanel (b). Finally, subpanel (f) demonstrates the lack of any additional magnetic field based switching up to 800 mT.

## S IV. EXTRACTING SPIN TRANSPORT CHARACTERISTICS

The general behavior of magnetic spin valves is well established [13–15]. The magnitude of switching, $dR_{NL} = dV_{NL}/I$, can be extracted from both lateral NL spin valve as well as Hanle spin precession measurement setups. The difference being that the field is applied along FM contact magnetization in the former case, leading to switching of the NL signal; while it is applied out-of-plane in the latter case, leading to spins in graphene precessing in-plane. Hanle spin precession is necessary to extract characteristics such as spin relaxation time. As described by Ref. [16], taking into account all paths between injector and detector in Eq. S2, considering diffusive motion, Larmor precession with frequency $\omega_L$, spin diffusion coefficient $D_S$ and spin relaxation with characteristic time $\tau_S$, results in curves similar to those experimentally obtained in Fig. S2 (c). The NL voltage at the detector can be described with:

$$\Delta V_{NL} \propto \int_0^{\infty} \frac{1}{4\pi t D_S} e^{-\frac{L^2}{4tD_S}} \cos(\omega_L t)\, e^{-\frac{t}{\tau_S}}. \tag{S2}$$

The proportionality constant is by definition the switching amplitude $dV_{NL}$ at $B_Z = 0$, expanded in the following analytical solution for Eq. S2:

$$V_{NL}(B) = \pm\gamma_i\gamma_d I \frac{R_{sq} D_S}{2W} \,\mathrm{Re}\left[\frac{e^{-L\sqrt{\frac{\omega}{D_S}}}}{\sqrt{\omega D_S}}\right], \tag{S3}$$

where $\gamma_i$ and $\gamma_d$ are the injector and detector contact interfacial spin polarizations, $R_{sq}$ the graphene sheet resistance, $\tau_S$, $D_S$ and $\lambda_S = \sqrt{\tau_S D_S}$ are spin relaxation time, spin diffusion coefficient and spin relaxation length in the graphene channel, $L$ and $W$ are the length and width of the channel, $I$ is the bias current used in the measurement, $\omega = \tau_S^{-1} - i\omega_L$ is a complex frequency, and $\pm$ denotes whether the injector and detector FM contacts are in a parallel or antiparallel magnetization configuration.

Despite the NL measurement configuration, the NL signal can have additional background features caused by stray charge currents [7, 17]. In our devices this may be more pronounced than usual due to the irregular shape of our exfoliated crystals and the resulting device geometries. Thus, a linear background needs to be considered along with Eq. S3. An example of this effect can be seen in the green curve of Fig. 2 (e) in the main text, where both the data as well as the black fitted line is noticeably not symmetric at larger $B_Z$ values. While accounting for such linear offset in the fitting, we can extract the relevant spin transport characteristics featured in Eq. S3. For the two devices in the main text, these values are summarized in Table II.

## S V. DETERMINATION OF INTERFACIAL CONTACT POLARIZATIONS

By using the spin transport characteristics obtained from the Hanle spin precession measurement, the interfacial spin polarization of the tunnel barriers used between FM and graphene can be calculated. Because our contact barrier resistances are similar to the graphene $R_{sq}$ (especially for Device 1), we can more accurately calculate the interfacial polarization of the injector-detector pair ($\gamma_i\gamma_d$) of the FM contacts by a modified expression containing the barrier resistance $R_b$, described by Ref. [18]:

| | $\tau_S$ | $D_S$ | $\lambda_S$ | $W$ | $R_{sq}$ |
|---|---|---|---|---|---|
| Units | ps | $cm^2s^{-1}$ | µm | µm | kΩ |
| Device 1 | $138 \pm 8$ | $93 \pm 4$ | $1.64 \pm 0.08$ | $1.3 \pm 0.1$ | $2.25 \pm 0.11$ |
| Device 2 | $545 \pm 20$ | $110 \pm 5$ | $2.44 \pm 0.10$ | $2.4 \pm 0.1$ | $1.20 \pm 0.06$ |

Table I. Spin transport characteristics of Device 1 and 2. $\tau_S$, $D_S$ and $\lambda_S$ are spin relaxation time, spin diffusion coefficient, and calculated spin relaxation length in the graphene channel, respectively. $W$ is the width of the graphene spin transport channel, $R_{sq}$ is the graphene sheet resistance.

| | $L$ | $R_b$ | $R_{INT}$ | $dR_{NL}$ | $\gamma_{FM}$ | $\gamma_{BiTeBr}$ |
|---|---|---|---|---|---|---|
| Units | µm | kΩ | kΩ | mΩ | % | % |
| Device 1 | | | | | | |
| Spin Valve | $3.9 \pm 0.2$ | $3.10 \pm 0.15$ | | $192 \pm 6$ | $3.4 \pm 0.3$ (C); $0.85 \pm 0.10$ (D) | |
| BiTeBr | $5.0 \pm 0.8$ | | $11 \pm 0.5$ | $10 \pm 1.0$ | $3.9 \pm 0.4$ (F) | $0.093 \pm 0.037$ |
| Device 2 | | | | | | |
| Spin Valve | $2.3 \pm 0.2$ | $14 \pm 0.5$ | | $810 \pm 30$ | $1.5 \pm 0.2$ | |
| BiTeBr | $5.1 \pm 0.9$ | | $8.3 \pm 0.4$ | $10 \pm 1.0$ | $1.5 \pm 0.2$ | $0.076 \pm 0.023$ |

Table II. Polarizations obtained from NL measurements of Device 1 and 2. $L$ is the length of the graphene spin transport channel for the particular measurement. $R_b$ is the $TiO_2$ tunnel barrier resistance of the FM contacts at zero bias. $R_{INT}$ is the BiTeBr to graphene interface resistance. $\gamma_{FM}$ gives the range of calculated polarizations of FM contacts. $\gamma_{BiTeBr}$ is the calculated $\gamma_i$ polarization when injecting spins from BiTeBr into graphene.

$$\gamma_i\gamma_d = \frac{dR_{NL}}{4R_b}\left[2\cosh\left(\frac{L}{\lambda_{NM}}\right) + \left(\frac{R_b}{R_{NM}} + \frac{R_{NM}}{R_b}\right)\sinh\left(\frac{L}{\lambda_{NM}}\right)\right], \tag{S4}$$

where $dR_{NL}$ is the jump in NL resistance in the spin valve measurement, and $R_{NM} = R_{sq}\frac{\lambda_{NM}}{W}$ is the spin resistance of the graphene channel, with $\lambda_{NM}$ the spin relaxation length. Note that applying the equation to any pair of FM contacts only results in a $\gamma_i\gamma_d$ combined polarization of the two contacts which can't normally be separated. However, for Device 1, sufficient separate pairwise measurements were taken to obtain the individual polarizations of each FM contact. For Device 2, we use the $\sqrt{\gamma_i\gamma_d}$ estimation for the polarizations. Obtaining the interfacial polarizations associated with spin injection originating from bulk BiTeBr was done using the same equation. In other words, the BiTeBr/interface/graphene structure was treated similarly to a FM/tunnel barrier/graphene structure. The BiTeBr-graphene interface resistance $R_{INT}$ was used instead of $R_b$, and the previously obtained FM polarization was substituted into $\gamma_d$. Table I contains the spin transport characteristics of the graphene in Device 1 and Device 2. The margin of error for $\tau_S$ and $D_S$ are from the fitting of Hanle curves, while $\lambda_S$ is calculated. $R_{sq}$ is obtained from four-terminal charge transport measurements. The NL measurements and interfacial polarizations obtained for the devices are shown in Table II. We note that for the regular spin valve measurements the error of $L$ comes from FM contact width and is reasonably low, while for the case of using BiTeBr as an injector we have chosen for error the half-width of the BiTeBr crystal covering the graphene. This margin of error is responsible for the relatively large uncertainty of $\gamma_{BiTeBr}$.

## S VI. ANGLE OF BITEBR-INJECTED SPIN POLARIZATION

The novel spin injection measurements are performed similarly to the NL spin valve and Hanle spin precession measurements, with the difference that a metallic top contact on BiTeBr and a distant reference contact on graphene are used for current biasing. This makes the BiTeBr crystal behave as the spin injector. As evidenced, the injected spin does not depend on the applied magnetic field $B_Y$, but is changed by changing the orientation of the bias current in the device. In the context of REE, spin polarization is generated perpendicular to the applied electric field. However, due to the irregular shape of the BiTeBr crystals and the nearby contact geometry, this electric field $E_{IP}$ doesn't necessarily point in the x-direction only, thus the injected spins will not point exactly in the y-direction either. FM contacts, however, are aligned in y-direction.

Performing Hanle spin precession on Device 1, in Fig. 4 of the main text, a slight asymmetry is observed in the obtained Hanle curves. This is caused by the aforementioned offset angle between injected spin polarization from BiTeBr and FM contact magnetization (parallel to $B_Y$) direction. The angle can be calculated in the following way.

The $\cos(\omega_L t)$ Larmor precession term in Eq. S2 describes a situation when spin is injected in a parallel or antiparallel orientation with respect to the detector. For a fully perpendicular spin polarization with respect to FM detector contacts, the term becomes $\sin(\omega_L t)$ and an antisymmetric Hanle curve is obtained. For an arbitrary offset angle $\phi$, depicted in Fig. 4 (a) in the main text, between injector and detector orientation, an analytical solution similar to Eq. S3 can be obtained:

$$V_{NL} = \pm\gamma_i\gamma_d I \frac{R_{sq}D_S}{2W}\left\{\cos\phi \,\mathrm{Re}\left[\frac{e^{-L\sqrt{\frac{\omega}{D_S}}}}{\sqrt{\omega D_S}}\right] + \sin\phi \,\mathrm{Im}\left[\frac{e^{-L\sqrt{\frac{\omega}{D_S}}}}{\sqrt{\omega D_S}}\right]\right\}. \tag{S5}$$

The effect of changing the angle $\phi$ is shown in the main text in Fig. 4 (c), with the Hanle curve smoothly shifting from a symmetric (blue) to an antisymmetric (green) one, in increments of 10 degrees. This allows the fitting of Eq. S5 to an experimental dataset to obtain an offset angle. The method has also recently been used in Ref. [19] to measure various injector-detector offset angles in a complex graphene geometry.

As shown in Fig. 4 (b) of the main text, in Device 1 this offset angle is obtained to be approximately 6°. In Device 2, using contacts T and V (see Fig. S2 (a)) in turn as top contact for vertical injection, offset angles of between 37° and 30° are obtained, respectively. This demonstrates that electrical control over spin orientation is possible: from the geometry of the top contacts and BiTeBr, we can expect biasing through contact T to produce a greater angle. A visual representation of the spin orientations due to electric field $E_{IP}$ in Device 2 can be seen in the inset of Fig. 4 (d) in the main text. These curves are visually different from the fully parallel (0°) Hanle curves, depicted on Fig. 4 (d) as a dashed black line for comparison. Therefore, using top contacts in different positions is expected to result in different offset angles, even for the same BiTeBr-graphene device. These angle offset measurements further support that the origin of the injected spin signal is the BiTeBr bulk.

## S VII. ELECTRIC FIELD INSIDE BITEBR

The BiTeBr crystals are 100 nm thick and several μm wide. Their resistance is also lower than that of either the interface or graphene. Intuitively, this suggests a predominantly in-plane electric field. To verify, we performed finite element electrostatic simulations, using COMSOL, on a simplified geometric model of a BiTeBr/graphene device, presented in Fig. S3. The simulation followed the dimensions and geometry of Device 2, with the BiTeBr thickness of

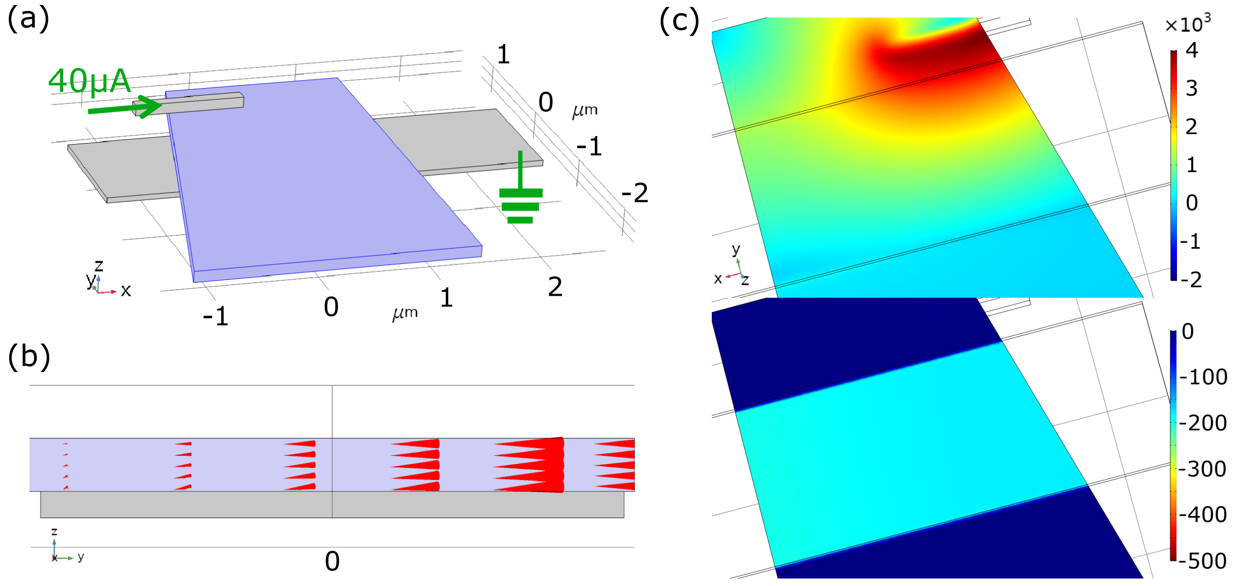


Figure S3. **COMSOL simulation of a BiTeBr/graphene device.** a) Geometry, with BiTeBr highlighted in light blue, a top metallic injector contact introducing a current of 40 μA, and the ground being defined on one end of the graphene. b) Cross section of the BiTeBr/graphene interface area, with cones showing the electric field orientation in BiTeBr, and the drop in magnitude of the electric field as more and more field enters the graphene. The field is predominantly in-plane. c) Color plots of in-plane (top) and out-of-plane (bottom) electric field magnitude in BiTeBr, seen from below.

100 μm, homogeneous interface resistance of 10 kΩ, and a geometry with an offset metallic top contact where a 40 μA bias current is injected, and the grounding contact in the graphene, as shown in panel a). A cross section of BiTeBr above the interface area, in panel b), depicts the overall direction of electric field inside the crystal. The dominance of the in-plane component is visible. In addition, it can be noted that there is little variation of the in-plane field along the z-axis coordinate, while the out-of-plane component increases closer to the interface. Finally, c) shows color plots of the in-plane (upper picture) and out-of-plane (lower picture) field components, seen from the bottom of the interface, where the graphene can be seen as a transparent black outline. The out-of-plane field component is homogeneous across the interface, and is of magnitude 180-200 V/m. The in-plane component ranges from approximately 3300 V/m closest to the metallic top contact, to below 100 V/m in the opposite edge of the interface. The area average is in the 800-1000 V/m range, and the magnitude remains larger than the out-of-plane component across almost the entire interface.

To simplify modeling, in the following we will work with the assumption of a fully in-plane field, neglecting the out-of-plane component. The field magnitude is also calculated from a simple resistance model using the bias current and the four-terminal resistance $R_{\mathrm{BiTeBr}} \approx 100\,\Omega$, resulting in 3000-3500 V/m, similar to the peak values obtained in the COMSOL simulation.

## S VIII. TUNNEL JUNCTION MODEL FOR BITEBR-GRAPHENE INTERFACE

The NL spin valve measurements are used to obtain the polarization of spin current, $\gamma_{\mathrm{i}}$, injected into graphene. This polarization originates from an imbalance of spin population in the BiTeBr. To determine the relationship between $\gamma_{\mathrm{i}}$ and bulk spin polarization in BiTeBr, the BiTeBr/graphene structure was modeled as a tunnel junction (see Fig. S4). The interface between the BiTeBr crystal and the graphene is a tunnel barrier and the tunneling current is

$$I = \frac{2\pi e}{\hbar} \int \mathrm{d}\xi_G \sum_{\mathbf{k}} \left\{ f^0(\xi_G) - f[\xi(\mathbf{k})] \right\} g(\xi_G) |M|^2 \delta \left[ \xi_G - \xi(\mathbf{k}) + eV \right], \tag{S6}$$

which after integrating becomes

$$I = \frac{2\pi e}{\hbar} \sum_{\mathbf{k}} \left\{ f^0[\xi(\mathbf{k}) - eV] - f[\xi(\mathbf{k})] \right\} g[\xi(\mathbf{k}) - eV] |M|^2, \tag{S7}$$

where $e$ is the elementary charge, $\hbar$ is the reduced Planck constant, $V$ is the voltage applied on the barrier and $M$ is the tunneling matrix element. $g$ is the density of states (DOS) of the graphene, $f^0$ is the Fermi function, $\xi_G$ is the energy measured from the Fermi level of graphene, $f$ is the distribution function of BiTeBr, $\xi(\mathbf{k}) = \epsilon_{\mathrm{BiTeBr}}(\mathbf{k}) - \mu_{\mathrm{BiTeBr}}$ is the energy measured from the Fermi level of BiTeBr, while for BiTeBr a 3D dispersion relation is used with anisotropic effective mass. The dispersion of the two Rashba-split subbands is:

$$\epsilon_{\mathrm{BiTeBr}}(\mathbf{k}) = \frac{\hbar^2 (k_x^2 + k_y^2)}{2m_\parallel} + \frac{\hbar^2 k_z^2}{2m_\perp} \pm \alpha_R \sqrt{k_x^2 + k_y^2}, \tag{S8}$$

where $m_\parallel = 0.15 m_{\mathrm{e}}$ (with $m_e$ the electron mass) is the in-plane effective mass in BiTeBr, and $m_\perp = 5 m_\parallel$ is the out-of-plane effective mass [20], $\alpha_R$ is the BiTeBr Rashba parameter, and the subbands are distinguished by the $\pm$ term. The summation in Eq. S7 runs over the occupied states in the $k$-space of the BiTeBr. The matrix element was chosen to be constant

$$|M|^2 = \frac{2\hbar^2}{m_e} |\Phi| e^{-\frac{2d}{\hbar}\sqrt{2m_e\Phi}}, \tag{S9}$$

where $\Phi$ and $d$ is the height and width of the tunnel barrier. The DOS of the graphene is

$$g(\epsilon) = \frac{2|\epsilon - \mu_{\mathrm{G}}|}{\pi \hbar^2 v_F^2}, \tag{S10}$$

where $v_F = 10^6$ m/s is the Fermi velocity in the graphene and $\mu_{\mathrm{G}}$ is the energy distance of the chemical potential from the Dirac point given by

$$\mu = \hbar v_F \sqrt{\pi n} = \hbar v_F \sqrt{\pi} \sqrt[4]{n_{\mathrm{RES}}^2 + \left( \frac{\epsilon_0 \epsilon_r |V|}{ed} \right)^2}, \tag{S11}$$

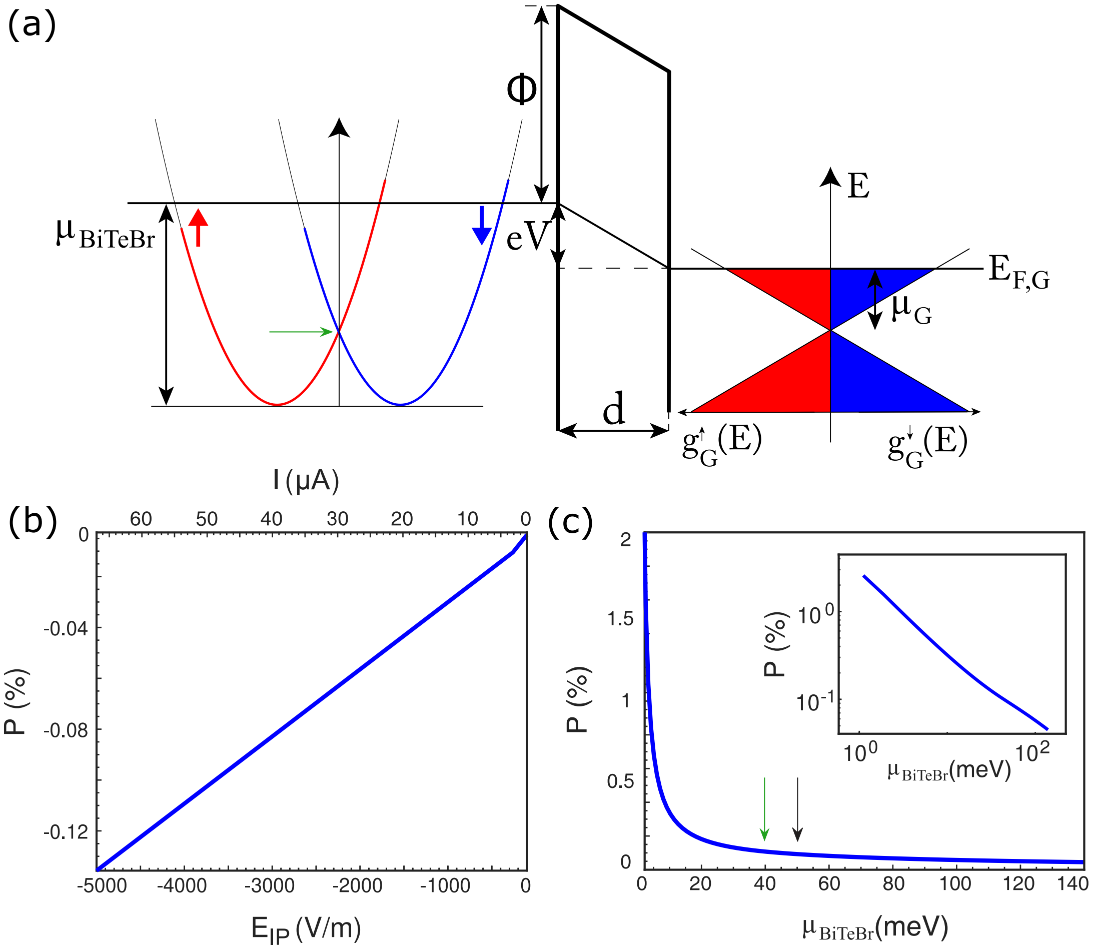


Figure S4. (a) Schematic picture of the tunneling model between the BiTeBr and the graphene. A 1D cross section of the BiTeBr conduction band is on the left, undergoing REE near $\mu_{\rm BiTeBr}$ due to applied electric field. The red and blue colors represent occupied states of the two opposing spin populations. On the right, states in graphene are represented, with filling up to $\mu_{\rm G}$, the Fermi level in the graphene. $\Phi$ and $d$ are the barrier height and width, and the voltage across the barrier is $V$. (b) Spin current polarization as a function of the electric field in the BiTeBr crystal, determined by the tunnel current, using the parameters mentioned in the text. Note that there is a linear dependence between $E_{\rm IP}$ and tunnel current, see the corresponding upper axis. (c) The polarization of the injected current as a function of chemical potential in BiTeBr. Inset: The same data in log-log scale. The curves show an inverse dependence $P \sim \mu_{\rm BiTeBr}^{-1}$, which ensures strong $P$ enhancement as $\mu_{\rm BiTeBr}$ is decreased. The green arrow indicates the location of the crossing of BiTeBr subbands, while the black arrow indicates the estimated position of $\mu_{\rm BiTeBr}$ in our BiTeBr crystals.

where $n_{\rm RES}$ is the residual charge density, $\epsilon_0$ is the vacuum permittivity and $\epsilon_r$ is the dielectric constant of the tunnel barrier. In our case, the voltage applied to the BiTeBr layer will also gate the graphene flake.

When an electric field is applied on the BiTeBr, it shifts the Fermi surface by $\mathbf{k_d} = -E_{\rm IP} e\tau/\hbar$, where $E_{\rm IP}$ is the electric field induced by the voltage drop in the BiTeBr crystal. We treat this via the distribution function of BiTeBr, $f$, which is the solution of the Boltzmann equation using a first order correction of the Fermi distribution function in the electric field $E_{\rm IP}$:

$$f(\epsilon) = f^0(\epsilon) - e\tau \mathbf{E}_{\rm IP}\mathbf{v}\frac{\partial f^0}{\partial \epsilon}, \tag{S12}$$

where $\mathbf{v} = \nabla_{\mathbf{k}}\epsilon/\hbar$ is the group velocity and $\tau$ is the momentum relaxation time in BiTeBr. This was estimated from the Drude model: $\tau = \frac{m_\parallel}{e^2 n_{\rm 3D}\rho_{\rm BiTeBr}}$. Using the BiTeBr resistivity of $10^{-5}$ Ωm, and charge carrier density of $10^{25}$ m$^{-3}$, we obtain an estimate $\tau = 5.3\times10^{-14}$ s; this value is similar to that obtained in Ref. [20]. The shift of the Fermi surface leads to a non-equilibrium spin density perpendicular to the applied electric field due to the helical spin structure of the BiTeBr (this is the REE). The helical spin structure of the dispersion relation of the BiTeBr can be taken into

account by a cosine function ($P = \cos[\arg(\mathbf{k})]$), then the spin dependent current is

$$I^\sigma = \frac{2\pi e}{\hbar} \sum_{\mathbf{k}} \left\{ f^0 \left[\xi(\mathbf{k}) - eV\right] - f\left[\xi(\mathbf{k})\right] \right\} g^\sigma[\xi(\mathbf{k}) - eV] P^\sigma(\mathbf{k}) |M|^2, \tag{S13}$$

where $\sigma$ stands for the $\uparrow$ or $\downarrow$ spin component in the perpendicular direction of the applied electric field and $g^\sigma$ is the half of $g$. The current polarization is given by

$$P = \frac{I^\uparrow - I^\downarrow}{I}. \tag{S14}$$

We note that, due to the helical spin texture of BiTeBr, $I \neq I^\uparrow + I^\downarrow$, as these denote a net polarization fully perpendicular to the applied field $E_{\mathrm{IP}}$.

Taking a fine grid in the 3D $k$-space of BiTeBr, the summation in Eq. S13 was carried out numerically with the following parameters used: $\Phi = 5\,\mathrm{eV}$, $d = 7.1\,\mathrm{Å}$, $\epsilon_r = 2$, $n_{\mathrm{RES}} = 5 \cdot 10^{15}\,\mathrm{m}^{-2}$, $R_{\mathrm{BiTeBr}} = 100\,\Omega$, $\alpha_{\mathrm{R}} = 2$ eVÅ, width of BiTeBr $w = 2.7\,\mu\mathrm{m}$, length $l = 5.5\,\mu\mathrm{m}$ and thickness $t \approx 100$ nm. Using a measured $n = 10^{25}\,\mathrm{m}^{-3}$ for the BiTeBr, the Fermi level $\mu_{\mathrm{BiTeBr}}$ is calculated from the BiTeBr dispersion. A value of $\approx 50\,\mathrm{meV}$, as measured from the bottom of the conduction bands, is obtained. The Fermi level is approximately 10 meV above the crossing point of the two subbands.

First the full tunnel current was calculated with respect to V, which was inverted to get the $V(I)$ dependence. Then, the electric field in the BiTeBr was calculated for the same current taking into account the resistance and geometry of the sample. Using finite $\mathbf{k_d}$ and Eq. S13 and Eq. S14, the spin polarization of the tunnel current, $P$, was calculated.

The calculated current polarizations with respect to the electric field are shown on Fig. S4 (b). The measurements were performed at a bias current of 40-80 µA, with corresponding electric field $E_{\mathrm{IP}}$ of 3000-3500 V/m for the different measurement configurations.

Fig. S4 (c) shows the Fermi level dependence of the current polarization at a fixed value of $E_{\mathrm{IP}} = 3500\,\mathrm{V/m}$. As the Fermi level is decreased closer to the bottom of the BiTeBr band, the current polarization is enhanced, with a dependence of approximately $P \sim \mu_{\mathrm{BiTeBr}}^{-1}$, which in case of a 3D dispersion relation is $P \sim n_{\mathrm{3D}}^{-2/3}$. Thus, with a decrease of the electron density in the BiTeBr conduction band, the current polarization can be strongly enhanced.

We also note here that the sign of polarization in graphene will always be the same as that in BiTeBr, regardless of current bias direction (the current bias direction will, however, determine BiTeBr polarization due to REE). This leads to the observed sign change in our experiments when, in a particular measurement configuration, we reverse the bias current, such as Fig. 3. (c) and (e) in the main text. We note here that this is a consequence of BiTeBr polarization being generated by a splitting of spin-dependent chemical potentials. Fig. S5 shows a simplified 1D cross section for the bands of BiTeBr and graphene, for both bias current directions. In the figure, the graphene bands are shown after the result of tunneling and relaxation, to highlight the resulting polarization. The dominant spin population in BiTeBr changes with bias direction, but due to the reversal of the voltage drop across the barrier, the interfacial current is polarized the same way for both bias directions. This results in the graphene always having the same polarization as the BiTeBr, regardless of whether spin injection or spin extraction is taking place. But the polarization reversal in the BiTeBr itself leads to the observed sign change.

This behavior is different from ferromagnetic contacts, where the sign of interfacial spin current polarization is given by a spin-dependent density of states at the Fermi level of the ferromagnet, and the spin-dependent chemical potential difference is negligible. When reversing bias current direction across a ferromagnet/graphene tunnel barrier, the polarization in graphene will flip, but that of the ferromagnet will stay the same.

## S IX. ESTIMATION OF REE AND SHE POLARIZATION

In the previous section, we calculated the expected polarization of current injected from BiTeBr into graphene. Here we will compare it to the experimental interfacial polarizations $\gamma_{\mathrm{i}}$ obtained using Eq. S4 previously, summarized in Table II.

In a material with Rashba spin-splitting, under the influence of an in-plane electric field the Fermi surface shifts in the direction of the field, leading to REE. The displacement $\mathbf{k_d}$ is linear with the electric field, and the resultant polarization is also linear with the electric field, as we saw in the previous sections. Our tunneling model also shows that polarization of interfacial spin current into graphene corresponds to the bulk REE polarization, and is inversely proportional to the Fermi level of the BiTeBr, $P_{\mathrm{REE}} \sim \mu_{\mathrm{BiTeBr}}^{-1}$. These observations are in agreement with REE theory [21].

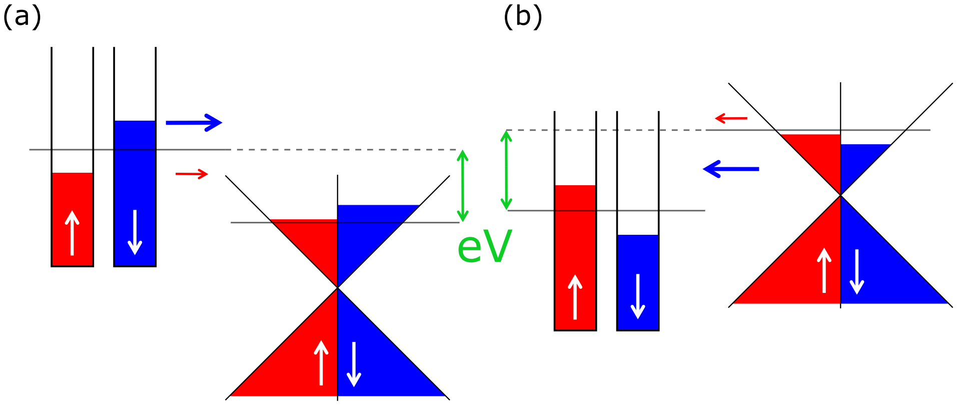


Figure S5. **Current bias reversal in tunneling model.** a) Spin injection into graphene: due to the electrochemical potential difference for spin up and down electrons in BiTeBr, the electrons transmitted through the bias window (between two dashed lines) result in spin down (blue) polarized electrons in graphene. b) Spin extraction from graphene, where more spin down electrons could tunnel from graphene to BiTeBr due to the electrochemical potential difference in BiTeBr, therefore graphene becomes spin up polarized. The graphene bands are shown after the tunneling process and relaxation, to highlight the resulting net polarization. In both cases graphene polarization is the same as REE-induced polarization in BiTeBr.

The values for the electric field in the BiTeBr, $E_{\mathrm{IP}}$, are estimated from the BiTeBr charge transport properties, bias current $I$, and geometry. The crystal thickness $t_{\mathrm{BiTeBr}}$ is obtained by AFM imaging. A simple estimation for $E_{\mathrm{IP}}$ can take into account distance $l$ between top contact and BiTeBr crystal edge (where it contacts graphene) towards the charge sink, as well as BiTeBr width $w$. From $E_{\mathrm{IP}} = RI/l = \rho I/(wt)$, using device geometry and bias currents used in the measurements, for Device 1 we obtain electric fields of 3500 V/m and 3000 V/m when detecting on contact D and F respectively (see Fig. 3 of main text). The experimentally observed polarizations $\gamma_{\mathrm{i}}$, from NL spin valve measurements, are 0.09 % and 0.07 % respectively. Consulting Fig. S4 (b), for these electric fields our model predicts polarizations of 0.095 % and 0.083 %, which is reasonably close to the experimental values. For Device 2 (see Fig. 4 of main text), a similar electric field of around 3000 V/m is obtained, and the experimentally obtained $\gamma_{\mathrm{i}} = 0.08\,\%$ is again close to the value predicted by the model.

Considering the polarization originates in the bulk, $\mu_{\mathrm{BiTeBr}} \sim n_{\mathrm{3D}}^{2/3}$ and thus $P_{\mathrm{REE}} \sim n_{\mathrm{3D}}^{-2/3}$. This provides a way to enhance $P_{\mathrm{REE}}$. Depending on growth conditions, variations in carrier density of an order of magnitude have already been reported [20, 22]. Producing BiTeBr crystals with a smaller thickness of 10-30 nm, significant carrier density tuning can be expected by back gate or ionic liquid gating techniques. Furthermore, with novel exfoliation techniques even single layer BiTeBr is within reach [23].

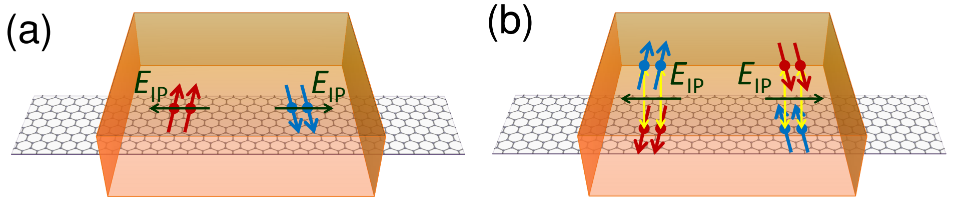


Figure S6. Illustration of spin polarization mechanisms REE and SHE. (a) An in-plane field $E_{\mathrm{IP}}$ in the flake produces a homogeneous polarization due to REE, with the shown orientation if the symmetry breaking out-of-plane field $E_{\mathrm{Z}}$ points upwards. (b) Horizontal Spin Hall Effect (SHE) produces homogeneous spin polarization at the bottom of the flake, which depends on the direction of $E_{\mathrm{IP}}$. An oppositely polarized spin layer is formed at the top of the flake. Shown here for the positive Spin Hall angle case, which opposes the REE polarization depicted in (a).

Aside from REE, the injected spin signal could also be the result of SHE within the BiTeBr crystal. However, in the following we argue that SHE cannot explain our experimental results. In case of SHE, a charge current within a material with large spin-orbit interaction (which is the case with BiTeBr) can produce a perpendicular spin current that leads to spin accumulation at the boundaries of the flake, within a region of thickness on the order of the spin relaxation length. Opposing boundaries would accumulate spins of opposing orientations, in contrast with REE where the entire material is polarized in the same orientation. This is depicted in Fig. S6.

To obtain the expected polarization at the edges of the BiTeBr flake through SHE only, we use the equation derived in Ref. [24] using a drift-diffusion approach assuming small electric fields, suitable for metallic or other low resistivity conductors, such as our BiTeBr. Using a 3D expression for the diffusion coefficient, with an anisotropic effective mass described by $m_\perp = 5m_\parallel$ (where $m_\parallel = 0.15m_\mathrm{e}$ is the in-plane effective mass of BiTeBr)[20], the following expression describes SHE polarization magnitude at the boundary layers of the BiTeBr crystal:

$$P_\mathrm{SHE} = \alpha_\mathrm{SHE}\lambda_\mathrm{S}\frac{e\sqrt{2\mu_\mathrm{BiTeBr}m_\perp}m_\parallel}{\pi^2\hbar^3 n_\mathrm{3D}}E_\mathrm{IP}, \tag{S15}$$

where $\alpha_\mathrm{SHE}$ is the Spin Hall angle, $\lambda_\mathrm{S}$ is the spin relaxation length in BiTeBr, $n_\mathrm{3D}$ is the 3D carrier density of BiTeBr, and $\mu_\mathrm{BiTeBr}$ is the Fermi level measured from the bottom of the conduction band, which in our case is approximately 50 meV. The polarization is proportional with the product of the spin Hall angle and spin relaxation length. The latter has not yet been measured for BiTeBr, however for a material with metallic behavior and very high SOI we could not expect it to be higher than of the order 10 nm. Also, since SHE describes a conversion from charge current to spin current, $\alpha_\mathrm{SHE} \leq 1$.

Eq. S15 can be rearranged the following way:

$$\alpha_{SHE} = \gamma_\mathrm{BiTeBr}\frac{1}{\lambda_\mathrm{S}}\frac{1}{E_\mathrm{IP}}\frac{\pi^2\hbar^3 n_\mathrm{3D}}{e\sqrt{2\mu_\mathrm{BiTeBr}m_\perp}m_\parallel}, \tag{S16}$$

where we have replaced $P_\mathrm{SHE}$ with the experimentally observed polarization $\gamma_\mathrm{BiTeBr}$. To obtain a lower bound estimate for $\alpha_{SHE}$ we use the highest reasonable values for $\lambda_\mathrm{S}$ (10 nm) and $E_\mathrm{IP}$. In previous sections we have also seen that the highest values for $E_\mathrm{IP}$ are in the range 3000-3500 V/m.

The third term in Eq. S16 scales with $n_\mathrm{3D}^{2/3}$, as $\mu_\mathrm{BiTeBr} \sim n_\mathrm{3D}^{2/3}$. From Hall measurements the carrier density of our BiTeBr samples is in the range 0.75-1.2 $\times 10^{25}$ m$^{-3}$, which also corresponds to a $\mu_\mathrm{BiTeBr}$ range of 41-56 meV. The lower value of 0.75 $\times 10^{25}$ m$^{-3}$ minimizes $\alpha_{SHE}$.

Using the experimentally obtained polarization values of 0.09 % for Device 1 and 0.08 % for Device 2 we obtain a lower bound for $\alpha_{SHE}$ of 1.25 for Device 1 and 1.11 for Device 2. On the other hand, by using the high end value for $n_\mathrm{3D}$ as well as the area average for $E_\mathrm{IP} \approx 900$ V/m obtained from COMSOL simulation, we obtain even larger values for $\alpha_{SHE}$ of 5.71 for Device 1 and 5.08 for Device 2. The conclusion is that, for an assumed $\lambda_\mathrm{S} \approx 10$ nm (which we consider to be a very reasonable upper bound), the required spin Hall angle $\alpha_{SHE}$ of BiTeBr that can explain the experimental observations is in the range 1.11-5.71. Since even the lower bound of this range is over-unity, we consider that SHE is a less likely origin for our experimental findings, and REE explains them better.

---


[1] K. A. Kokh, B. G. Nenashev, A. E. Kokh, and G. Y. Shvedenkov, Journal of Crystal Growth **275**, 2129 (2005).
[2] U. Petasch, C. Hennig, and H. Oppermann, Zeitschrift für Naturforschung **54b**, 234 (1999).
[3] I. Y. Sklyadneva, R. Heid, K.-P. Bohnen, V. Chis, V. A. Volodin, K. A. Kokh, O. E. Tereshchenko, P. M. Echenique, and E. V. Chulkov, Physical Review B **86**, 094302 (2012).
[4] H. Zhong, Z. Zhang, H. Xu, C. Qiu, and L.-M. Peng, AIP Advances **5**, 057136 (2015).
[5] A. Avsar, J. Y. Tan, T. Taychatanapat, J. Balakrishnan, G. Koon, Y. Yeo, J. Lahiri, A. Carvalho, A. S. Rodin, E. O'Farrell, and et al., Nature Communications **5**, 4875 (2014).
[6] C. K. Safeer, J. Ingla-Aynés, F. Herling, J. H. Garcia, M. Vila, N. Ontoso, M. R. Calvo, S. Roche, L. E. Hueso, and F. Casanova, Nano Letters **19**, 1074 (2019).
[7] T. S. Ghiasi, A. A. Kaverzin, P. J. Blah, and B. J. van Wees, Nano Letters **19**, 5959–5966 (2019).
[8] B. Zhao, D. Khokhriakov, Y. Zhang, H. Fu, B. Karpiak, A. M. Hoque, X. Xu, Y. Jiang, B. Yan, and S. P. Dash, Phys. Rev. Research **2**, 013286 (2020).
[9] W. Han, K. McCreary, K. Pi, W. Wang, Y. Li, H. Wen, J. Chen, and R. Kawakami, Journal of Magnetism and Magnetic Materials **324**, 369–381 (2012).
[10] T. Maassen, I. J. Vera-Marun, M. H. D. Guimarães, and B. J. van Wees, Phys. Rev. B **86**, 235408 (2012).
[11] F. Volmer, M. Drögeler, G. Güntherodt, C. Stampfer, and B. Beschoten, Synthetic Metals **210**, 42 (2015).
[12] P. J. Zomer, M. H. D. Guimarães, N. Tombros, and B. J. van Wees, Phys. Rev. B **86**, 161416 (2012).
[13] J. Fabian, A. Matos-Abiague, C. Ertler, P. Stano, and I. Žutić, Acta Physica Slovaca. Reviews and Tutorials **57**, 565 (2007).
[14] W. Han, R. K. Kawakami, M. Gmitra, and J. Fabian, Nature Nanotechnology **9**, 794–807 (2014).
[15] S. Takahashi and S. Maekawa, Physica C: Superconductivity **437-438**, 309 (2006).
[16] F. J. Jedema, M. V. Costache, H. B. Heersche, J. J. A. Baselmans, and B. J. van Wees, Applied Physics Letters **81**, 5162–5164 (2002).

[17] A. Dankert and S. Dash, Nature Communications **8**, 16093 (2017).
[18] T. Valet and A. Fert, Phys. Rev. B **48**, 7099 (1993).
[19] D. Khokhriakov, B. Karpiak, A. M. Hoque, and S. P. Dash, Carbon **161**, 892 (2019).
[20] T. Ideue, K. Hamamoto, S. Koshikawa, M. Ezawa, S. Shimizu, Y. Kaneko, Y. Tokura, N. Nagaosa, and Y. Iwasa, Nature Physics **13**, 578 (2017).
[21] V. M. Edelstein, Solid State Communications **73**, 233 (1990).
[22] M. Kanou and T. Sasagawa, Journal of Physics: Condensed Matter **25**, 135801 (2013).
[23] B. Fülöp, Z. Tajkov, J. Pető, P. Kun, J. Koltai, L. Oroszlány, E. Tóvári, H. Murakawa, Y. Tokura, S. Bordács, L. Tapasztó, and S. Csonka, 2D Materials **5**, 031013 (2018).
[24] M. I. Dyakonov, Future Trends in Microelectronics , 251 (2010), arXiv:1210.3200.
